# Supplementary material for: Mitigating Cache Noise in Test-Time Adaptation for Large Vision-Language Models
Source: arXiv:2503.18334 source file (2025-03-31)
Supplement: Supplementary file 1 [file supp_ood.tex]

\begin{table*}[ht]

\caption{\textbf{Performance comparisons on robustness to natural distribution shifts}. We present top-1 accuracy (\%) results for all evaluated methods employing both ResNet-50 and ViT-B/16 visual backbones of CLIP. Additionally, we assess the performance using prompts learned by CoOp~\cite{zhou2022learning} with 16-shot training data per class on ImageNet~\cite{deng2009imagenet}. The best results are highlighted in \textbf{bold}.}
\vspace{5pt}
  \centering
  \resizebox{\linewidth}{!}{
  \begin{tabular}{lccccccc}
    \toprule
    {Method}      & ImageNet   &  ImageNet-A  &  ImageNet-V2  & ImageNet-R 
    & ImageNet-S   
    &{Average}  & {OOD Average}     \\
  \midrule
  CLIP-ResNet-50~\cite{radford2021learning}       &58.16&	21.83&	51.41	&56.15	&33.37&	44.18&	40.69           \\ 
  \midrule
  Ensemble          &  59.81&	23.24&	52.91	&{60.72}	&35.48&	46.43&	43.09  \\
  TPT~\cite{shu2022test}          &  60.74 & 26.67  &    54.70   &  59.11   &  35.09   &    47.26    &     43.89    \\
  DiffTPT~\cite{feng2023diverse} & 60.80 & \textbf{31.06} & 55.80 & 58.80 & 37.10 & 48.71 & 45.69 \\
  TDA~\cite{karmanov2024efficient} & 61.35 & 30.29 & 55.54 & 62.58 & 38.12 & 49.58 & 46.63 \\ \rowcolor{gray!20}
  \textbf{Ours} & \textbf{63.41} & 30.15 & \textbf{56.72} & \textbf{63.72} & \textbf{40.03} & \textbf{50.81}  & \textbf{47.66} \\ \rowcolor{gray!20}
   & ($\pm$ 0.23) & ($\pm$ 0.41) & ($\pm$ 0.22) & ($\pm$ 0.20) & ($\pm$ 0.11) & ($\pm$ 0.21)  & ($\pm$ 0.22) \\
  \midrule
  CoOp~\cite{zhou2022learning}            &  63.33 &  23.06  &   55.40     &  56.60   &  34.67   &     46.61   &     42.43       \\
    TPT + CoOp~\cite{shu2022test}           &  64.73  & 30.32  & 57.83       &  58.99   &  35.86   &   49.55     &   45.75\\
  DiffTPT + CoOp~\cite{feng2023diverse}           &  64.70  & \textbf{32.96}  & \textbf{61.70}       &  58.20   &  36.80   &   \textbf{50.87}     &   \textbf{47.42} \\ \rowcolor{gray!20}
  % TDA + CoOp$^\dag$~\cite{karmanov2024efficient} & 62.71 & 29.96 & 55.75 & 59.76 & \textbf{38.02} & 49.24 & 45.87 \\ \rowcolor{gray!20}
\textbf{Ours + CoOp} & \textbf{64.86} & 30.08 & 57.96 & \textbf{59.78} & \textbf{37.80} & 50.10 & 46.41 \\ \rowcolor{gray!20}
   & ($\pm$ 0.18) & ($\pm$ 0.27) & ($\pm$ 0.31) & ($\pm$ 0.19) & ($\pm$ 0.17) & ($\pm$ 0.22)  & ($\pm$ 0.23) \\
  \midrule
  \midrule
  CLIP-ViT-B/16~\cite{radford2021learning}       & 66.73&	47.87&	60.86&	73.98&	46.09&	59.11&	57.20             \\
  \midrule
  Ensemble          &  68.34&	49.89&	61.88&	{77.65}&	48.24&	61.20&	59.42  \\
  TPT~\cite{shu2022test}           &  68.98  & 54.77  & 63.45       &  77.06   &  47.94   &   62.44     &   60.81 \\
  DiffTPT~\cite{feng2023diverse}           &  70.30  & 55.68  & 65.10       &  75.00   &  46.80   &   62.28     &   60.52 \\
  TDA~\cite{karmanov2024efficient} & 69.51 & \textbf{60.11} & 64.67 & 80.24 & 50.54 & 65.01 & 63.89 \\ \rowcolor{gray!20}
  \textbf{Ours} & \textbf{71.91} & 59.63 & \textbf{65.44} & \textbf{80.40} & \textbf{52.26} & \textbf{65.93} & \textbf{64.43} \\ \rowcolor{gray!20}
   & ($\pm$ 0.09) & ($\pm$ 0.18) & ($\pm$ 0.17) & ($\pm$ 0.24) & ($\pm$ 0.11) & ($\pm$ 0.16)  & ($\pm$ 0.18) \\
  \midrule
  CoOp~\cite{zhou2022learning}          &  71.51 &  49.71  &   64.20     &  75.21   &  47.99   &   61.72     &   59.28  \\
  TPT + CoOp~\cite{shu2022test}           &  73.61  & 57.95  & \textbf{66.83}       &  77.27   &  49.29   &   64.99     &   62.83 \\
  DiffTPT + CoOp~\cite{feng2023diverse}           &  \textbf{75.00}  & 58.09  & 66.80       &  73.90   &  49.50   &   64.12     &   61.97 \\ \rowcolor{gray!20}
  % TDA + CoOp$^\dag$~\cite{karmanov2024efficient} & 71.13 & \textbf{59.83} & 64.81& \textbf{79.73} & 50.74 & 65.25 &  \\ \rowcolor{gray!20}
\textbf{Ours + CoOp} & 73.67 & \textbf{59.43} & 66.38 & 78.49 & \textbf{50.78} & \textbf{65.75} & \textbf{63.77} \\ \rowcolor{gray!20}
   & ($\pm$ 0.14) & ($\pm$ 0.36) & ($\pm$ 0.32) & ($\pm$ 0.06) & ($\pm$ 0.08) & ($\pm$ 0.23)  & ($\pm$ 0.26) \\
    \bottomrule
  \end{tabular}
    }
\label{tab:ood-supp}
\end{table*}
